# Supplementary material for: Anisotropic electrostatic screening of charged colloids in nematic solvents
Source: arXiv:2005.05682 ancillary file (2021-01-28)
Supplement: Supplementary file 1 [file SI_aniso.pdf]

# Supplementary Materials: Anisotropic electrostatic screening of charged colloids in nematic solvents

Jeffrey C. Everts,<sup>1,2,\*</sup> Bohdan Senyuk,<sup>3,\*</sup> Haridas Mundoor,<sup>3</sup> Miha Ravnik,<sup>1,4,†</sup> and Ivan I. Smalyukh<sup>3,5,6,‡</sup>

<sup>1</sup>*Faculty of Mathematics and Physics, University of Ljubljana, Jadranska 19, 1000 Ljubljana, Slovenia.*

<sup>2</sup>*Institute of Physical Chemistry, Polish Academy of Sciences, Kasprzaka 44/52, PL-01-224 Warsaw, Poland*

<sup>3</sup>*Department of Physics and Soft Materials Research Center,  
University of Colorado, Boulder, CO 80309, USA.*

<sup>4</sup>*Jozef Stefan Institute, Jamova 39, 1000 Ljubljana, Slovenia.*

<sup>5</sup>*Department of Electrical, Computer, and Energy Engineering,  
Materials Science and Engineering Program, University of Colorado, Boulder, CO 80309, USA.*

<sup>6</sup>*Renewable and Sustainable Energy Institute, National Renewable Energy Laboratory,  
University of Colorado, Boulder, CO 80309, USA.*

(Dated: December 24, 2020)

---

\* These two authors contributed equally

† [miha.ravnik@fmf.uni-lj.si](mailto:miha.ravnik@fmf.uni-lj.si)

‡ [ivan.smalyukh@colorado.edu](mailto:ivan.smalyukh@colorado.edu)

# DERIVATION OF THE ANISOTROPIC POISSON-BOLTZMANN EQUATION AND THE EFFECTIVE PAIR POTENTIAL

Consider two charged colloidal bodies with degrees of freedom  $\Omega_i$ ,  $i = 1, 2$  in a system volume  $V$ , which labels the center-of-mass position  $\mathbf{R}_i$  and orientational degrees of freedom. We assume the particles to carry a constant charge density  $\sigma$ . Outside the particles ions described by their density profiles  $\rho_{\pm}(\mathbf{r})$  are immersed in a nematic medium with dielectric tensor  $\epsilon_{ij}(\mathbf{r})$ . The particles occupy a volume  $\Gamma_i$ , with surface  $\partial\Gamma_i$ . We consider the free energy functional,

$$\beta\mathcal{F}[\rho_{\pm}, \phi; \Omega_1, \Omega_2] = \int_V d\mathbf{r} \left[ q(\mathbf{r})\phi(\mathbf{r}) - \frac{1}{8\pi\lambda_B} \epsilon_{ij}(\mathbf{r}) \partial_i \phi(\mathbf{r}) \partial_j \phi(\mathbf{r}) \right] + \sum_{\alpha=\pm} \int_V d\mathbf{r} \rho_{\alpha}(\mathbf{r}) \{ \log[\rho_{\alpha}(\mathbf{r})\Lambda_{\alpha}^3] - 1 \}, \quad (\text{S.1})$$

where  $\beta^{-1} = k_B T$  is the thermal energy,  $\lambda_B = e^2/(4\pi\epsilon_0 k_B T)$  is the Bjerrum length in vacuum with  $\epsilon_0$  the vacuum permittivity and  $e$  the elementary charge. Finally  $\phi(\mathbf{r})/(\beta e)$  is the electrostatic potential and here taken as a variational parameter. We take the following external potential  $V_{\text{ext}}(\mathbf{r})$  for the ions

$$V_{\text{ext}}(\mathbf{r}) = \begin{cases} \infty, & \mathbf{r} \in \Gamma_1 \cup \Gamma_2, \\ 0, & \mathbf{r} \notin \Gamma_1 \cup \Gamma_2, \end{cases} \quad (\text{S.2})$$

which encodes the fact that ions cannot penetrate the hard cores of the particles. The Euler-Lagrange equations for the ion densities can straightforwardly be found by using the relation

$$\frac{\delta\mathcal{F}}{\delta\rho_{\pm}} = \mu_{\pm} - V_{\text{ext}}(\mathbf{r}), \quad (\text{S.3})$$

with  $\beta\mu_{\pm} = \log(\rho_{\pm}\Lambda_{\pm}^3)$  the reservoir chemical potential (taken as ideal gas) and  $\rho_s$  the reservoir cation/anion density. In the particular case, where we consider only two particles in a macroscopic system volume  $V$ ,  $\rho_s$  equals the bulk ion densities. We find

$$\rho_{\pm}(\mathbf{r}) = \rho_s \exp[\mp\phi(\mathbf{r}) - \beta V_{\text{ext}}(\mathbf{r})]. \quad (\text{S.4})$$

The electrostatic potential can then be found via the Poisson equation, which is obtained from the Euler-Lagrange equation  $\delta\mathcal{F}/\delta\phi(\mathbf{r}) = 0$ ,

$$-\partial_i[\epsilon_{ij}(\mathbf{r})\partial_j\phi(\mathbf{r})] = 4\pi\lambda_B q(\mathbf{r}), \quad (\text{S.5})$$

with  $q(\mathbf{r})$  the total net charge density. In the specific example where the two charged bodies are identical spheres with radius  $a$ , we have  $q(\mathbf{r}) = \rho_+(\mathbf{r}) - \rho_-(\mathbf{r}) + \sigma \sum_i \delta(|\mathbf{r} - \mathbf{R}_i| - a)$ . In the definition for  $\epsilon_{ij}(\mathbf{r})$  outside of the particles, it is convenient to scale out the quantity  $\bar{\epsilon} = \text{Tr}(\epsilon)/3$ , which is the dielectric constant in the case of no orientational ordering at that specific temperature. We specify

$$\epsilon_{ij}(\mathbf{r}) = \begin{cases} \bar{\epsilon}[\tilde{\epsilon}_{\perp} \delta_{ij} + \Delta\tilde{\epsilon} n_i(\mathbf{r}) n_j(\mathbf{r})], & \mathbf{r} \notin \Gamma_1 \cup \Gamma_2, \\ \epsilon_p \delta_{ij}, & \mathbf{r} \in \Gamma_1 \cup \Gamma_2, \end{cases} \quad (\text{S.6})$$

with  $\Delta\tilde{\epsilon} = \tilde{\epsilon}_{\parallel} - \tilde{\epsilon}_{\perp}$  and  $\mathbf{n}(\mathbf{r})$  the director field of the liquid crystalline medium, which we assume to be fixed. Finally,  $\epsilon_p$  is the dielectric constant of the particle. Combining Eq. (S.4) with Eq. (S.5) we find the Poisson-Boltzmann (PB) equation outside the particles,

$$\partial_i[\tilde{\epsilon}_{ij}\partial_j\phi(\mathbf{r})] = \kappa^2 \sinh[\phi(\mathbf{r})], \quad \mathbf{r} \in V \setminus (\Gamma_1 \cup \Gamma_2), \quad (\text{S.7})$$

with  $\kappa^{-1} = \lambda_D^I = (8\pi\lambda_B^I \rho_s)^{-1/2}$  the Debye screening length for the isotropic case, and  $\lambda_B^I = \lambda_B/\bar{\epsilon}$ . Inside the particles, we find the Laplace equation,

$$\nabla^2\phi(\mathbf{r}) = 0, \quad \mathbf{r} \in \Gamma_1 \cup \Gamma_2, \quad (\text{S.8})$$

complemented by boundary conditions (obtained from the surface terms in the Euler-Lagrange equation for  $\phi(\mathbf{r})$ ),

$$\hat{\nu}_i[\epsilon_{ij}\partial_j\phi(\mathbf{r})|_{\Gamma^+} - \epsilon_p\partial_i\phi(\mathbf{r})|_{\Gamma^-}] = 4\pi\lambda_B\sigma, \quad \mathbf{r} \in \Gamma_i, \quad i = 1, 2, \quad (\text{S.9})$$

$$\hat{\nu} \cdot \nabla\phi(\mathbf{r}) = 0, \quad \mathbf{r} \in \partial V, \quad (\text{S.10})$$

with  $\hat{\nu}$  an outward-pointing unit normal. The effective pair potential is

$$H(\Omega_1, \Omega_2) = \phi_{\text{HC}}(\Omega_1, \Omega_2) + \min_{\rho_{\pm}, \phi} \left\{ \mathcal{F}[\rho_{\pm} \phi; \Omega_1, \Omega_2] - \sum_{\alpha} \int d\mathbf{r} \rho_{\alpha}(\mathbf{r}) [\mu_{\pm} - V_{\text{ext}}(\mathbf{r})] \right\}, \quad (\text{S.11})$$

with hard-core potential  $\phi_{\text{HC}}(\Omega_1, \Omega_2) = \infty$  for  $\Gamma_1 \cap \Gamma_2 \neq \emptyset$ , and zero otherwise. Ultimately, we find

$$\beta H(\Omega_1, \Omega_2) = \beta \phi_{\text{HC}}(\Omega_1, \Omega_2) + \rho_s \int_{\mathcal{R}} d\mathbf{r} \left\{ \phi(\mathbf{r}) \sinh \phi(\mathbf{r}) - 2[\cosh \phi(\mathbf{r}) - 1] \right\} + \frac{1}{2} \sum_{i=1}^2 \int_{\Gamma_i} d\mathbf{r} \sigma \phi(\mathbf{r}). \quad (\text{S.12})$$

We subtracted a term extensive in the free volume for convenience.

### GREEN'S FUNCTION

Let us assume that  $|\phi(\mathbf{r})| \ll 1$ , and that  $\tilde{\epsilon}_{ij}$  is spatially constant. In this case the PB equation becomes the linearised PB equation using  $\sinh \phi \approx \phi$ . We can determine the Green's function  $G(\mathbf{r} - \mathbf{r}')$  for the linearised PB equation

$$[\partial_i(\tilde{\epsilon}_{ij}\partial_j) - \kappa^2] G(\mathbf{r} - \mathbf{r}') = -4\pi\delta(\mathbf{r} - \mathbf{r}') \quad (\text{S.13})$$

This equation is solved by a coordinate transformation  $s'_i = (\tilde{\epsilon}_{ij})^{-1/2}(r_j - r'_j)$ , which is well-defined since  $\tilde{\epsilon}$  is a symmetric positive-definite matrix. Using the chain rule  $\partial_i = \epsilon_{ij}^{-1/2}\partial'_j$  in Eq. (S.13), we find

$$(\nabla'^2 - \kappa^2)G(\mathbf{s}') = -4\pi\delta(\boldsymbol{\epsilon}^{1/2} \cdot \mathbf{s}'). \quad (\text{S.14})$$

Because of the transformation law for the delta function we obtain  $\delta(\boldsymbol{\epsilon}^{1/2} \cdot \mathbf{s}') = \delta(\mathbf{s}')/\sqrt{\det \tilde{\epsilon}}$ . Eq. (S.14) can easily be solved by Fourier transformation, followed by a contour integration to find the Fourier inverse. The result is

$$G(\mathbf{s}') = \frac{\exp(-\kappa|\mathbf{s}'|)}{\sqrt{\det \tilde{\epsilon}}|\mathbf{s}'|}. \quad (\text{S.15})$$

Then  $|\mathbf{s}'| = \sqrt{s'_i s'_i} = \sqrt{\epsilon_{ij}^{-1/2} \epsilon_{ik}^{-1/2} (r_j - r'_j)(r_k - r'_k)} = \sqrt{\epsilon_{ij}^{-1} (r_i - r'_i)(r_j - r'_j)}$ , to find

$$G(\mathbf{r} - \mathbf{r}') = \frac{\exp[-\kappa \sqrt{(\tilde{\epsilon}^{-1})_{ij} (r_i - r'_i)(r_j - r'_j)}]}{\sqrt{\det \tilde{\epsilon} (\tilde{\epsilon}^{-1})_{ij} (r_i - r'_i)(r_j - r'_j)}}. \quad (\text{S.16})$$

It is straightforward to check for isotropic systems,  $\tilde{\epsilon}_{ij} = \delta_{ij}$ , and the Green's function reduces to the standard Yukawa form.

We set  $\mathbf{n} = \mathbf{e}_z$ , then

$$G(\mathbf{r}, \mathbf{r}') = \frac{1}{\sqrt{\tilde{\epsilon}_{\perp}^2 \tilde{\epsilon}_{\parallel}}} \frac{\exp\left\{-\kappa \sqrt{[(x-x')^2 + (y-y')^2]/\tilde{\epsilon}_{\perp} + (z-z')^2/\tilde{\epsilon}_{\parallel}}\right\}}{\sqrt{[(x-x')^2 + (y-y')^2]/\tilde{\epsilon}_{\perp} + (z-z')^2/\tilde{\epsilon}_{\parallel}}}. \quad (\text{S.17})$$

The electrostatic potential for any charge distribution  $q(\mathbf{r})$  that is penetrable for ion is then given by

$$\phi(\mathbf{r}) = \lambda_{\text{B}}^{\text{I}} \int d\mathbf{r}' q(\mathbf{r}') G(\mathbf{r}, \mathbf{r}') \quad (\text{S.18})$$

### SPHERICAL-SHELL APPROXIMATION FOR ELECTROSTATIC POTENTIAL

In this section, we will show within linear theory that we can map an ion-impenetrable charged sphere on an ion-penetrable charged spherical shell, but with a renormalised surface charge density and radius. For a spherical shell of radius  $R$  and constant surface charge density  $\sigma_{\text{S}}$ , we have  $q(\mathbf{r}) = \sigma_{\text{S}}\delta(r - R)$ . The electrostatic potential then reads

$$\phi(r, \theta) = \frac{\sigma_{\text{S}} \lambda_{\text{B}} R^2}{\sqrt{\tilde{\epsilon}_{\perp}^2 \tilde{\epsilon}_{\parallel}}} \int_0^{2\pi} d\phi' \int_0^{\pi} d\theta' \sin \theta' \frac{\exp\left(-\kappa \sqrt{f_{\rho}/\tilde{\epsilon}_{\perp} + f_z/\tilde{\epsilon}_{\parallel}}\right)}{\sqrt{f_{\rho}/\tilde{\epsilon}_{\perp} + f_z/\tilde{\epsilon}_{\parallel}}}, \quad (\text{S.19})$$

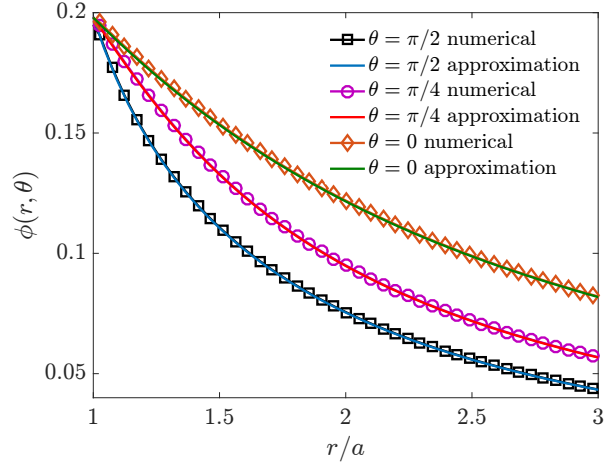

Figure S1. Electrostatic potential for  $\kappa a = 0.1$  calculated numerically and compared with the result of a spherical charged shell with  $\sigma_S = \sigma$  and  $R = a$ . In this example the charge is  $4\pi a^2 \sigma = 20$ .

with coefficients

$$f_\rho = r^2 \sin^2 \theta + R^2 \sin^2 \theta' - 2rR \cos \phi' \sin \theta \sin \theta', \quad (\text{S.20})$$

$$f_z = r^2 \cos^2 \theta + R^2 \cos^2 \theta' - 2rR \cos \theta \cos \theta'. \quad (\text{S.21})$$

We will now demonstrate that Eq. (S.19) represents the electrostatic potential of a charged sphere of radius  $a > R$  and charge density  $\sigma$ , given suitable values of  $\sigma_S$  and  $R$ , where the validity of Eq. (S.19) has to be taken  $r > a$ . We restrict ourselves to low charge densities to ensure that we are in the linear regime, we use  $4\pi a^2 \sigma = 20$ . In the case of a large Debye length,  $\kappa a = 0.1$ , there is hardly any renormalisation of the parameters. Namely, comparison between the numerical finite-element result and Eq. (S.19) using  $R = a$  and  $\sigma_S = \sigma$ , reveal that the two methods agree well for all distances and angles from the spherical particle, see Fig. S1.

This is an important result, because this method allows us to derive a semi-analytical expression in terms of a double integral for the electrostatic potential that is described otherwise by a very complicated differential equation. However, would we use this method also to describe the effective pair potential between two charged spheres, then there will be four integrations which are computationally more costly. It is therefore worthwhile to derive far-field results of the electrostatic potential, and Eq. (S.19) can be used as a starting point for deriving a far-field expansion similar to the well-known multipole expansion known for charge distributions in vacuum.

For shorter Debye lengths, the bare parameters of the particle cannot be used because the surface potential becomes highly inhomogeneous. However, it turns out that the angle dependence of the surface potential can be captured by Eq. (S.19), and even match the numerical result quite accurately by using  $\sigma_S$  and  $R$  as fitting parameters to the numerical obtained surface potential. This procedure is highlighted for  $\kappa a = 5$  in Fig. S2a, where we tune  $\sigma_S$  and  $R$  to match the surface potential of the particle. It turns out that the accuracy of Eq. (S.19) using these fitted parameters describe the electrostatic potential fairly accurately for almost all  $r$ , with only a small deviation close to the particle surface.

## MULTIPOLE EXPANSION FOR ELECTROSTATIC POTENTIAL

We derive a multipole expansion for ion-penetrable charge distributions  $q(\mathbf{r})$ , where the electrostatic potential is given by Eq. (S.18). We use the Cartesian representation, but it can be rather directly converted also to the spherical or cylindrical representation of the multipole expansion. For this, we expand  $G(\mathbf{r}, \mathbf{r}')$  as

$$G(\mathbf{r}, \mathbf{r}') = G(\mathbf{r}, 0) + G_i(\mathbf{r})x'_i + \frac{1}{2!}G_{ij}(\mathbf{r})x'_i x'_j + \frac{1}{3!}G_{ijk}(\mathbf{r})x'_i x'_j x'_k + \frac{1}{4!}G_{ijkl}(\mathbf{r})x'_i x'_j x'_k x'_l + \dots, \quad (\text{S.22})$$

with Einstein summation convention implied and coefficients are defined by

$$G_{i_1 \dots i_n}(\mathbf{r}) = \frac{\partial^n}{\partial x'_{i_1} \dots \partial x'_{i_n}} G(\mathbf{r}, \mathbf{r}') \Big|_{\mathbf{r}'=0}. \quad (\text{S.23})$$

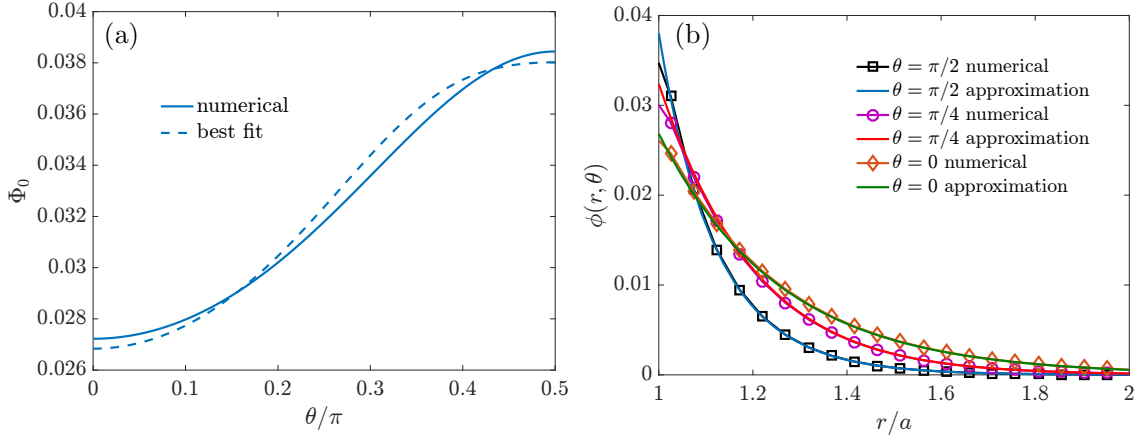

Figure S2. **a** Fitting procedure for  $\kappa a = 5$ .  $\sigma_S$  and  $R$  are tuned to match the numerically obtained surface potential. The result is  $R/a = 0.9662$  and  $\sigma_S = 2.0614\sigma$ , with  $4\pi a^2 \sigma = 20$ . **b** Comparison of electrostatic potential by using a spherical shell with renormalized parameters with the numerically calculated result for a charged sphere. The match between these two methods is excellent, except for very close to the particle.

The electrostatic potential is then

$$\phi(\mathbf{r}) = \lambda_B^I \left[ G(\mathbf{r}, 0) \int d\mathbf{r}' q(\mathbf{r}') + G_i(\mathbf{r}) \int d\mathbf{r}' x'_i q(\mathbf{r}') + \frac{1}{2!} G_{ij}(\mathbf{r}) \int d\mathbf{r}' x'_i x'_j q(\mathbf{r}') + \dots \right] \quad (\text{S.24})$$

For  $q(\mathbf{r}') = \sigma_S \delta(r' - R)$ , we find that

$$\int d\mathbf{r}' (x')^k (y')^l (z')^m q(\mathbf{r}') = 0, \quad (\text{S.25})$$

for either  $k, l$  or  $m$  odd, because of symmetry reasons. Note that in contrast to the bare Coulomb case, the quadrupole tensor cannot be chosen to be traceless, since  $G_{ij}$  is not traceless. We compute the non-zero components of the quadrupole tensor,

$$\int d\mathbf{r}' (x')^2 \delta(r' - R) = \int d\mathbf{r}' (y')^2 \delta(r' - R) = \int d\mathbf{r}' (z')^2 \delta(r' - R) = \frac{4}{3} \pi R^4. \quad (\text{S.26})$$

The components of the hexadecapole tensor are

$$\int d\mathbf{r}' (x')^4 \delta(r' - R) = \int d\mathbf{r}' (y')^4 \delta(r' - R) = \int d\mathbf{r}' (z')^4 \delta(r' - R) = \frac{4}{5} \pi R^6, \quad (\text{S.27})$$

$$\int d\mathbf{r}' (x')^2 (y')^2 \delta(r' - R) = \int d\mathbf{r}' (y')^2 (z')^2 \delta(r' - R) = \int d\mathbf{r}' (x')^2 (z')^2 \delta(r' - R) = \frac{4}{15} \pi R^6. \quad (\text{S.28})$$

The electrostatic potential then reads

$$\begin{aligned} \phi(\mathbf{r}) = \sigma_S \lambda_B^I \left\{ 4\pi R^2 G(\mathbf{r}, 0) + \frac{1}{2!} [G_{xx}(\mathbf{r}) + G_{yy}(\mathbf{r}) + G_{zz}(\mathbf{r})] \frac{4}{3} \pi R^4 + \right. \\ \left. \frac{1}{4!} [G_{xxxx}(\mathbf{r}) + G_{yyyy}(\mathbf{r}) + G_{zzzz}(\mathbf{r})] \frac{4}{5} \pi R^6 + \frac{1}{4!} [6G_{xxyy}(\mathbf{r}) + 6G_{yyzz}(\mathbf{r}) + 6G_{xxzz}(\mathbf{r})] \frac{4}{15} \pi R^6 + \dots \right\} \end{aligned} \quad (\text{S.29})$$

This can be rewritten as

$$\phi(\mathbf{r}) = 4\pi R^2 \sigma_S \lambda_B^I \left[ G_m(\mathbf{r}) + \frac{1}{6} R^2 G_q(\mathbf{r}) + \frac{1}{120} R^4 G_h(\mathbf{r}) + \dots \right], \quad (\text{S.30})$$

where we define the monopolar basis function

$$G_m(\mathbf{r}) = \frac{1}{\sqrt{\tilde{\epsilon}_\perp^2 \tilde{\epsilon}_\parallel}} \frac{\exp \{ -\kappa \sqrt{\rho^2 / \tilde{\epsilon}_\perp + z^2 / \tilde{\epsilon}_\parallel} \}}{\sqrt{\rho^2 / \tilde{\epsilon}_\perp + z^2 / \tilde{\epsilon}_\parallel}}. \quad (\text{S.31})$$

Moreover, the quadrupolar basis function is

$$G_q(\mathbf{r}) = G_{xx}(\mathbf{r}) + G_{yy}(\mathbf{r}) + G_{zz}(\mathbf{r}), \quad (\text{S.32})$$

or written in cylindrical coordinates with  $P = (\tilde{\epsilon}_\perp)^{-1}$ ,  $Q = (\tilde{\epsilon}_\parallel)^{-1}$  and  $|\mathbf{u}| = \sqrt{P\rho^2 + Qz^2}$ ,

$$G_q(\rho, z) = \frac{1}{\sqrt{\tilde{\epsilon}_\perp^2 \tilde{\epsilon}_\parallel}} \frac{e^{-\kappa|\mathbf{u}|}}{|\mathbf{u}|^5} \left\{ \kappa^2 P^3 \rho^4 + P^2 \rho^2 (\kappa^2 Q z^2 + \kappa|\mathbf{u}| + 1) + Q^2 z^2 (\kappa^2 Q z^2 + 2\kappa|\mathbf{u}| + 2) + \right. \\ \left. PQ \left[ \rho^2 (\kappa^2 Q z^2 - \kappa|\mathbf{u}| - 1) - 2z^2 (\kappa|\mathbf{u}| + 1) \right] \right\}. \quad (\text{S.33})$$

Finally, the hexadecapolar basis function is

$$G_h(\mathbf{r}) = G_{xxxx}(\mathbf{r}) + G_{yyyy}(\mathbf{r}) + G_{zzzz}(\mathbf{r}) + 2G_{xxyy}(\mathbf{r}) + 2G_{yyzz}(\mathbf{r}) + 2G_{xxzz}(\mathbf{r}), \quad (\text{S.34})$$

and expressed in cylindrical coordinates,

$$G_h(\rho, z) = \frac{1}{\sqrt{\tilde{\epsilon}_\perp^2 \tilde{\epsilon}_\parallel}} \frac{e^{-\kappa|\mathbf{u}|}}{|\mathbf{u}|^9} \left\{ \kappa^4 P^6 \rho^8 + \kappa^2 P^5 \rho^6 (2\kappa^2 Q z^2 + 2\kappa|\mathbf{u}| + 5) + P^4 \rho^4 \left[ \kappa^4 Q^2 z^2 (2\rho^2 + z^2) - \right. \right. \\ \left. - 2\kappa^3 Q (\rho^2 + 3z^2) |\mathbf{u}| - \kappa^2 Q (8\rho^2 + 27z^2) + 9\kappa|\mathbf{u}| + 9 \right] + P^3 Q \rho^2 \left[ 3\kappa^2 Q \rho^4 \right. \\ \left. - 8z^2 (\kappa^3 Q z^2 |\mathbf{u}| + 3\kappa^2 Q z^2 + 9\kappa|\mathbf{u}| + 9) + 2\rho^2 (2\kappa^4 Q^2 z^4 + 6\kappa^3 Q z^2 |\mathbf{u}| + 27\kappa^2 Q z^2 - 9\kappa|\mathbf{u}| - 9) \right] \\ \left. + P^2 Q^2 \left[ 8z^4 (\kappa^2 Q z^2 + 3\kappa|\mathbf{u}| + 3) + 2\rho^2 z^2 (\kappa^4 Q^2 z^4 + 5\kappa^3 Q z^2 |\mathbf{u}| + 21\kappa^2 Q z^2 + 72\kappa|\mathbf{u}| + 72) \right. \right. \\ \left. + \rho^4 (\kappa^4 Q^2 z^4 - 6\kappa^3 Q z^2 |\mathbf{u}| - 27\kappa^2 Q z^2 + 9\kappa|\mathbf{u}| + 9) \right] + Q^4 z^4 (\kappa^4 Q^2 z^4 + 4\kappa^3 Q z^2 |\mathbf{u}| + 12\kappa^2 Q z^2 \\ \left. + 24\kappa|\mathbf{u}| + 24) + 2PQ^3 z^2 \left[ \rho^2 (\kappa^4 Q^2 z^4 - \kappa^3 Q z^2 |\mathbf{u}| - 9\kappa^2 Q z^2 - 36\kappa|\mathbf{u}| + 36) \right. \right. \\ \left. \left. - 2z^2 (\kappa^3 Q z^2 |\mathbf{u}| + 5\kappa^2 Q z^2 + 12\kappa|\mathbf{u}| + 12) \right] \right\}. \quad (\text{S.35})$$

In the isotropic limit we have  $G_m(r) = \exp(-\kappa r)/r$ ,  $G_q(r) = \kappa^2 \exp(-\kappa r)/r$  and  $G_h(r) = \kappa^4 \exp(-\kappa r)/r$ . Recall however that  $R = R(\kappa)$  and  $\sigma_S = \sigma_S(\kappa)$ , so the series Eq. (S.30) is not resummed to  $\exp(\kappa R)/(1 + \kappa R)$ , which would have been the DLVO result.

Because the spherical-shell formula (S.19) represents the full numerical solution quite accurately, it suffices to just compare Eq. (S.19) with the multipole result Eq. (S.30). The prefactor is the same in both expressions, so we can check the accuracy by considering the reduced electrostatic potential

$$\phi(\mathbf{r}) = \frac{4\pi R^2 \sigma_S \lambda_B^I}{\sqrt{\tilde{\epsilon}_\perp^2 \tilde{\epsilon}_\parallel}} \tilde{\phi}(\mathbf{r}). \quad (\text{S.36})$$

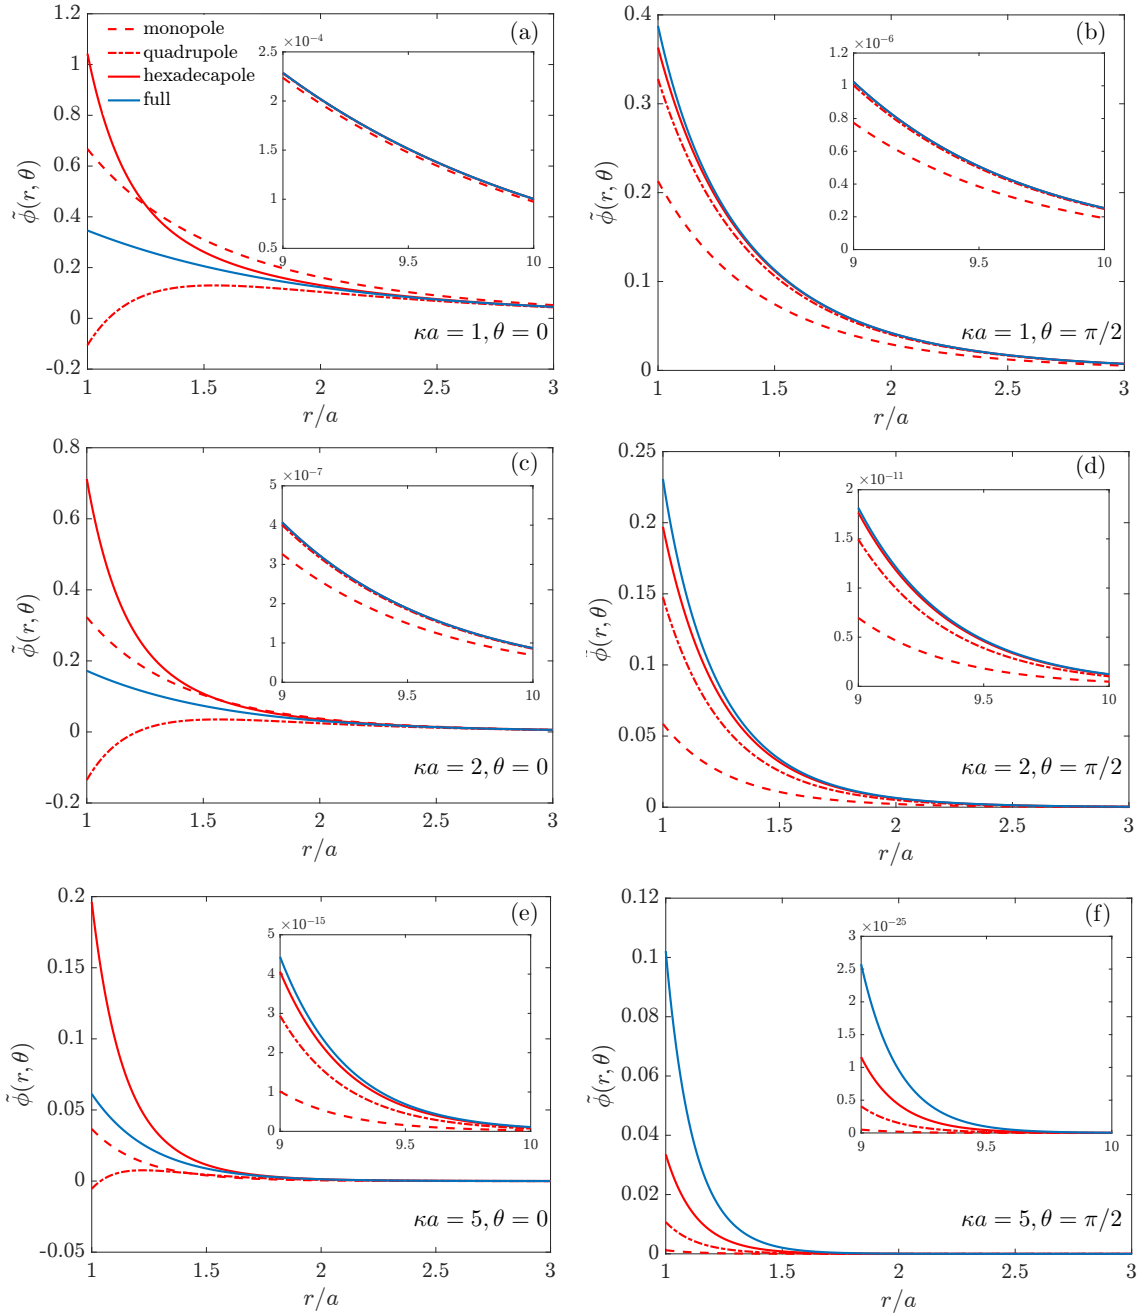

Figure S3. Comparison of the reduced electrostatic potential (see Eq. S.36) by using the spherical-shell representation (in blue) and the multipole expansion of this result (in red). We compare these results for various values of  $\kappa a$  and  $\theta$ , but also comparison of just including the monopolar term (dashed), up until the quadrupolar contribution (dot dashed), and up until hexadecapolar contribution (full). In the inset we show a comparison for distances asymptotically far from the particle.

In Fig. S3 this comparison is shown for various  $\kappa a$  and  $\theta$ . For all parameter values there is a disagreement between the full result and the multipole expansion for short distances similar to the multipole expansion in vacuum. Additionally, higher order terms are needed to describe the results for high values of  $\kappa a$ . For  $\kappa a = 1$  (Fig. S3a, b) it suffices to use the terms up until quadrupolar order and even the multipole is sufficient for small angles  $\theta \approx 0$ , see Fig. S3a. Increasing  $\kappa a$  means that we need higher order terms to describe the solution accurately, for  $\kappa a = 2$  (Fig. S3c, d) we need up until hexadecapolar (full line), while clearly for  $\theta = \pi/2$  the quadrupolar term is insufficient even asymptotically far from the particle. Finally, for  $\kappa a = 5$  even up until hexadecapolar order is not sufficient, see Figs. S3e and S3f.

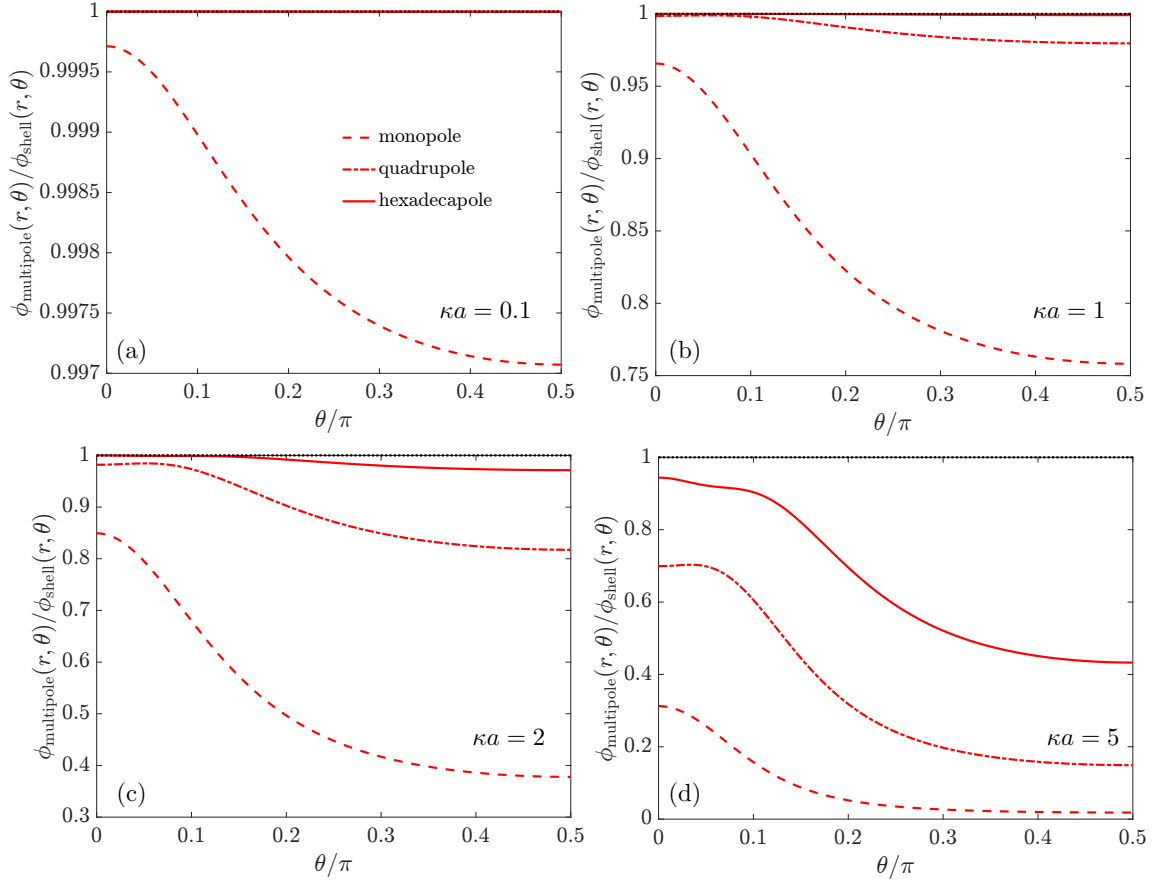

Figure S4. Far-field angle dependence comparison of the electrostatic potential for  $r/a = 1 + 10/\kappa$ . When the result equals unity the match is exact.

In Fig. S4 we compare the angle dependence of the electrostatic potential for the shell method and its multipole expansion “asymptotically” far from the particle. Surprisingly, even asymptotically far from the particle, we cannot describe the electrostatic potential of the charged sphere by a point charge for sufficiently large  $\kappa a$ . This result is well known for anisotropic particles, where this anisotropy that still persists at “infinity” is described by the so-called anisotropy function. We see that this effect is also present in the case of an isotropic particle but in an anisotropic medium. However, the result is more profound, not only the prefactor becomes angle dependent (as is described by the anisotropy function), but also the screening length.

#### SPHERICAL-SHELL APPROXIMATION FOR EFFECTIVE PAIR INTERACTION

The spherical-shell method of the previous section allows us to derive analytical expressions for the effective pair interaction between two charged spheres. Within the linear superposition approximation the effective pair interaction is

$$\beta\Phi(\mathbf{R}_1, \mathbf{R}_2) = \int d\mathbf{r} q^{(1)}(\mathbf{r}; \mathbf{R}_1) \phi^{(2)}(\mathbf{r}; \mathbf{R}_2), \quad (\text{S.37})$$

where  $\phi^{(2)}(\mathbf{r}; \mathbf{R}_2) = \phi(\mathbf{r} - \mathbf{R}_2)$  is the single-particle electrostatic potential for particle 2 situated with centre of mass at  $\mathbf{r} = \mathbf{R}_2$  and  $q^{(1)}(\mathbf{r}; \mathbf{R}_1) = \sigma_S \delta(|\mathbf{r} - \mathbf{R}_1| - R)$ . By a coordinate transformation  $\mathbf{r} \rightarrow \mathbf{r} + \mathbf{R}_1$  and defining  $\mathbf{X} = \mathbf{R}_1 - \mathbf{R}_2$  we find

$$\beta\Phi(\mathbf{R}_1, \mathbf{R}_2) = \int d\mathbf{r} q^{(1)}(\mathbf{r}) \phi(\mathbf{r} + \mathbf{X}), \quad (\text{S.38})$$

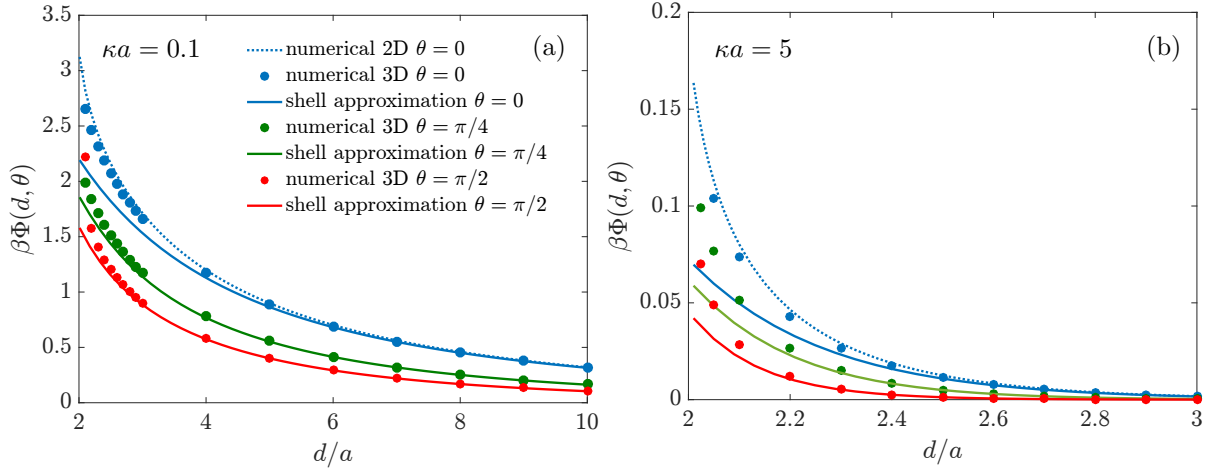

Figure S5. Comparison of numerical finite-element result with spherical-shell renormalisation procedure + linear superposition approximation for the effective pair interaction between two charged spheres. The comparison is made for  $4\pi a^2 \sigma = 20$ ,  $a/\lambda_B = 100$ ,  $\tilde{\epsilon}_{\parallel} = 1.9$  and  $\tilde{\epsilon}_{\perp} = 0.6$ . To assess the quality of the numerical COMSOL code in 3D, we also added for  $\theta = 0$  the result from a 2D COMSOL calculation which allows for finer meshes (dashed blue line). For  $R$  and  $\sigma_S$  we use the same values as in Fig. S2.

which with the help of Eq. (S.18) can be rewritten as

$$\beta\Phi(\mathbf{X}) = \lambda_B^I \int d\mathbf{r}' \int d\mathbf{r}'' q^{(1)}(\mathbf{r}') G(\mathbf{r}' + \mathbf{X}, \mathbf{r}'') q^{(2)}(\mathbf{r}''). \quad (\text{S.39})$$

Now we specialise to two spherical charged shells, then

$$\beta\Phi(\mathbf{X}) = \frac{\sigma_S^2 R^4 \lambda_B^I}{\sqrt{\tilde{\epsilon}_{\perp}^2 \tilde{\epsilon}_{\parallel}}} \int_0^{2\pi} d\phi' \int_0^{\pi} d\theta' \sin \theta' \int_0^{2\pi} d\phi'' \int_0^{\pi} \sin \theta'' \frac{\exp[-\kappa \sqrt{F_{\rho}/\tilde{\epsilon}_{\perp} + F_z/\tilde{\epsilon}_{\parallel}}]}{\sqrt{F_{\rho}/\tilde{\epsilon}_{\perp} + F_z/\tilde{\epsilon}_{\parallel}}} \quad (\text{S.40})$$

with

$$F_{\rho} = d^2 \sin^2 \theta + 2dR \cos(\phi - \phi') \sin \theta \sin \theta' + R^2 \sin^2 \theta' - 2dR \cos(\phi - \phi'') \sin \theta \sin \theta'' - 2R^2 \cos(\phi' - \phi'') \sin \theta' \sin \theta'' + R^2 \sin^2 \theta'', \quad (\text{S.41})$$

and

$$F_z = R^2 \cos^2 \theta' - 2R^2 \cos \theta' \cos \theta'' + R^2 \cos^2 \theta'' + 2dR \cos \theta' \cos \theta - 2dR \cos \theta'' \cos \theta + d^2 \cos^2 \theta, \quad (\text{S.42})$$

where we have parametrised  $\mathbf{X} = (d \cos \phi \sin \theta, d \sin \phi \sin \theta, d \cos \theta)$ . Note that  $\Phi(\mathbf{X}) = \Phi(d, \theta)$ .

We compare the pair potential obtained from the spherical-shell method and the linear superposition approximation (LSA) with the full numerical result in Fig. S5. For large screening lengths the shell method converges for even distances smaller than the screening length to the numerical result, see Fig. S5a comparison of the filled circles with the full lines. In contrast, for  $\kappa a = 5$  the shell+LSA method represents the numerical solution after roughly one Debye length. The fact that the LSA performs less well for higher values of  $\kappa a$  is quite well known even for isotropic systems.

## MULTIPOLE EXPANSION FOR EFFECTIVE PAIR INTERACTION

Similar to the multipole expansion for the electrostatic potential, we can use Eq. (S.39) to find a far-field expansion for the effective pair interaction. We start by Taylor expanding the electrostatic potential around the centre of the second particle,

$$\phi(\mathbf{r} + \mathbf{X}) = \phi(\mathbf{X}) + \phi_i(\mathbf{X}) x_i + \frac{1}{2!} \phi_{ij}(\mathbf{X}) x_i x_j + \frac{1}{3!} \phi_{ijk}(\mathbf{X}) x_i x_j x_k + \frac{1}{4!} \phi_{ijkl}(\mathbf{X}) x_i x_j x_k x_l + \dots, \quad (\text{S.43})$$

where

$$\phi_{i_1 \dots i_n}(\mathbf{X}) = \frac{\partial^n}{\partial x_{i_1} \dots \partial x_{i_n}} \phi(\mathbf{r} + \mathbf{X}) \Big|_{\mathbf{r}=0}. \quad (\text{S.44})$$

We note the following property

$$\frac{\partial}{\partial x_j} G_i(\mathbf{r} + \mathbf{X}) \Big|_{\mathbf{r}=0} = \frac{\partial}{\partial x_j} \left( \frac{\partial}{\partial x'_i} G(\mathbf{r} + \mathbf{X}, \mathbf{r}') \Big|_{\mathbf{r}'=0} \right) \Big|_{\mathbf{r}=0} = - \left( \frac{\partial^2}{\partial x'_i \partial x'_j} G(\mathbf{r} + \mathbf{X}, \mathbf{r}') \right) \Big|_{\mathbf{r}=\mathbf{r}'=0} = -G_{ij}(\mathbf{X})$$

The pair interaction decomposes as (note all odd moments vanish by symmetry),

$$\Phi(\mathbf{X}) = \Phi_{\text{MM}}(\mathbf{X}) + \Phi_{\text{MQ}}(\mathbf{X}) + \Phi_{\text{QM}}(\mathbf{X}) + \Phi_{\text{QQ}}(\mathbf{X}) + \Phi_{\text{MH}}(\mathbf{X}) + \Phi_{\text{HM}}(\mathbf{X}) + \dots \quad (\text{S.45})$$

We have the monopole-monopole interaction

$$\beta\Phi_{\text{MM}}(\mathbf{X}) = \lambda_{\text{B}}^{\text{I}} G(\mathbf{X}, 0) \int d\mathbf{r} q^{(1)}(\mathbf{r}) \int d\mathbf{r}' q^{(2)}(\mathbf{r}'). \quad (\text{S.46})$$

Compare this expression with the expression for two point charges. The monopole-quadrupole interactions are

$$\beta\Phi_{\text{MQ}}(\mathbf{X}) = \frac{\lambda_{\text{B}}^{\text{I}}}{2!} G_{ij}(\mathbf{X}) \int d\mathbf{r} q^{(1)}(\mathbf{r}) \int d\mathbf{r}' x'_i x'_j q^{(2)}(\mathbf{r}'), \quad (\text{S.47})$$

$$\beta\Phi_{\text{QM}}(\mathbf{X}) = \frac{\lambda_{\text{B}}^{\text{I}}}{2!} G_{ij}(\mathbf{X}) \int d\mathbf{r} x_i x_j q^{(1)}(\mathbf{r}) \int d\mathbf{r}' q^{(2)}(\mathbf{r}'), \quad (\text{S.48})$$

The quadrupole-quadrupole interaction is

$$\beta\Phi_{\text{QQ}}(\mathbf{X}) = \frac{\lambda_{\text{B}}^{\text{I}}}{2!2!} G_{ijkl}(\mathbf{X}) \int d\mathbf{r} x_i x_j q^{(1)}(\mathbf{r}) \int d\mathbf{r}' x'_k x'_l q^{(2)}(\mathbf{r}'), \quad (\text{S.49})$$

and finally the monopole-hexadecapole interactions

$$\beta\Phi_{\text{MH}}(\mathbf{X}) = \frac{\lambda_{\text{B}}^{\text{I}}}{4!} G_{ijkl}(\mathbf{X}) \int d\mathbf{r} q^{(1)}(\mathbf{r}) \int d\mathbf{r}' x'_i x'_j x'_k x'_l q^{(2)}(\mathbf{r}'), \quad (\text{S.50})$$

$$\beta\Phi_{\text{HM}}(\mathbf{X}) = \frac{\lambda_{\text{B}}^{\text{I}}}{4!} G_{ijkl}(\mathbf{X}) \int d\mathbf{r} x_i x_j x_k x_l q^{(1)}(\mathbf{r}) \int d\mathbf{r}' q^{(2)}(\mathbf{r}'). \quad (\text{S.51})$$

Note that all the multipoles are defined with respect to the centre of mass frame of the particles. All expressions up until now are general. Now we will take for the two charge distributions a spherical shell with charge density  $\sigma_{\text{S}}$ . We find

$$\beta\Phi_{\text{MM}}(\mathbf{X}) = \lambda_{\text{B}}^{\text{I}} (4\pi R^2 \sigma_{\text{S}})^2 G_{\text{m}}(\mathbf{X}), \quad (\text{S.52})$$

$$\beta\Phi_{\text{MQ}}(\mathbf{X}) = \beta\Phi_{\text{QM}}(\mathbf{X}) = \frac{\lambda_{\text{B}}^{\text{I}}}{2!} G_q(\mathbf{X}) (\sigma_{\text{S}} 4\pi R^2) \left( \sigma_{\text{S}} \frac{4}{3} \pi R^4 \right), \quad (\text{S.53})$$

$$\beta\Phi_{\text{QQ}}(\mathbf{X}) = \frac{\lambda_{\text{B}}^{\text{I}}}{2!2!} G_h(\mathbf{X}) \left( \sigma_{\text{S}} \frac{4}{3} \pi R^4 \right)^2, \quad (\text{S.54})$$

$$\beta\Phi_{\text{MH}}(\mathbf{X}) = \beta\Phi_{\text{HM}}(\mathbf{X}) = \frac{\lambda_{\text{B}}^{\text{I}}}{4!} G_h(\mathbf{X}) (\sigma_{\text{S}} 4\pi R^2) \left( \sigma_{\text{S}} \frac{4}{5} \pi R^6 \right), \quad (\text{S.55})$$

We note that e.g.  $G_{m,q,h}(\mathbf{X}) = G_{m,q,h}(d \sin \theta, d \cos \theta)$ , so that the expressions of Section IV (Eqs. (S.31), (S.33), (S.35)) can be used directly. The final expression up until monopole-hexadecapole is

$$\beta\Phi(\mathbf{X}) = \lambda_{\text{B}}^{\text{I}} (4\pi \sigma_{\text{S}} R^2)^2 \left[ G_{\text{m}}(\mathbf{X}) + \frac{1}{3} G_q(\mathbf{X}) R^2 + \frac{2}{45} G_h(\mathbf{X}) R^4 + \dots \right], \quad (\text{S.56})$$

where we recall that  $\sigma_{\text{S}} = \sigma_{\text{S}}(\sigma, \kappa a)$  and  $R = R(\sigma, \kappa a)$ , have to be found by fitting the surface potential, as has been described before.

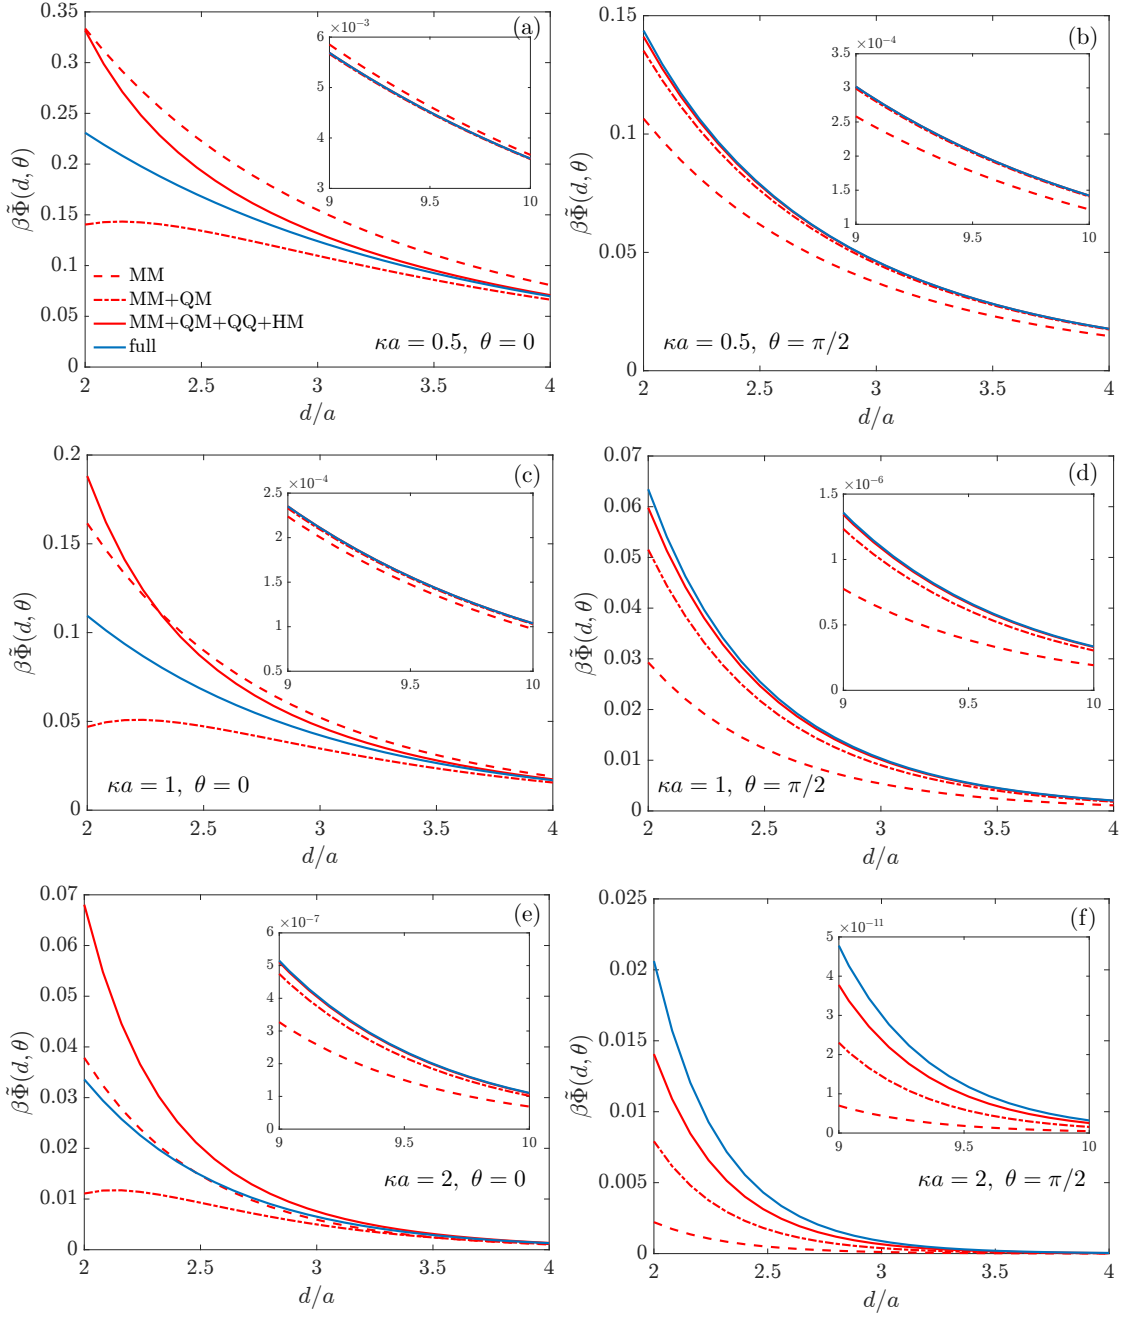

Figure S6. Comparison of the reduced effective pair potential (see Eq. (S.57)) by using the spherical-shell representation (in blue) and the multipole expansion of this result (in red). We compare these results for various values of  $\kappa a$  and  $\theta$ , but also comparison of just including the monopole-monopole contribution (dashed), with the monopole-quadrupolar contribution added (dot dashed), and up until quadrupole-quadrupole and hexadecapole-monopole terms (full). In the inset we show a comparison for distances asymptotically far from the particle.

We compare the multipole result with the spherical shell+LSA approximation in Fig. S6 by plotting the reduced effective pair interaction  $\tilde{\Phi}(\mathbf{X})$  given by

$$\beta\Phi(\mathbf{X}) = \frac{\lambda_B^I}{\sqrt{\tilde{\epsilon}_\perp^2 \tilde{\epsilon}_\parallel}} (4\pi\sigma_S R^2)^2 \beta\tilde{\Phi}(\mathbf{X}). \quad (\text{S.57})$$

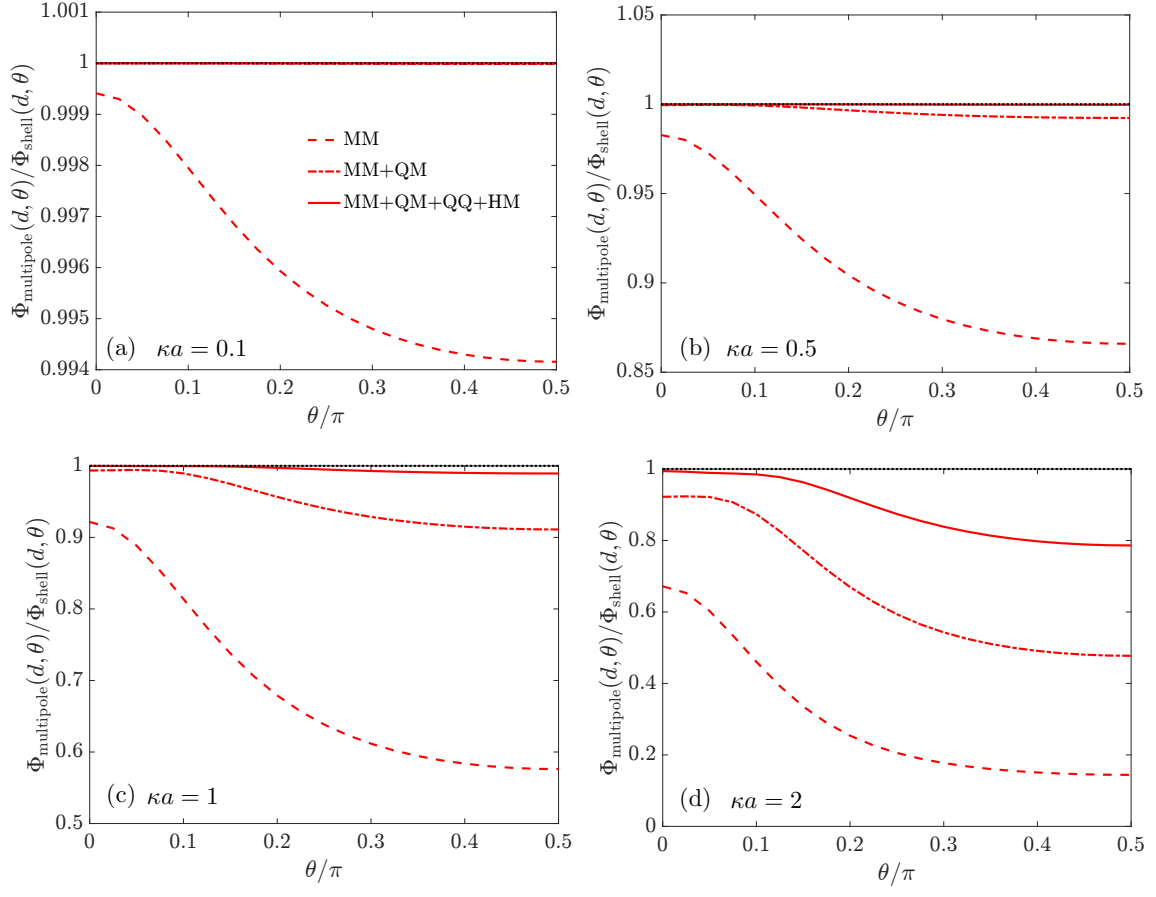

Figure S7. Far-field angle dependence comparison of the effective pair potential for  $d/a = 2 + 10/\kappa$ . When the result equals unity the match is exact.

Similar to the description of the electrostatic potential in terms of Yukawa multipoles, we see that higher order terms are needed in order to describe the effective pair interaction at high values of  $\kappa a$ . The only difference, however, seems to be that the validity of the expansion is for lower values of  $\kappa a$  than the result of the electrostatic potential. Whereas up until the hexadecapole could describe the electrostatic potential at  $\kappa a = 2$  almost indistinguishably, see Figs. S3c and S3d, up until the hexadecapole-monopole and quadrupole-monopole terms seem to break down already at  $\kappa a = 2$  for the effective pair interaction, see Fig. S6f. This is reflected for the interaction asymptotically far from the particle for every angle, see Fig. S7.

## SUPPLEMENTARY EXPERIMENTAL FIGURES

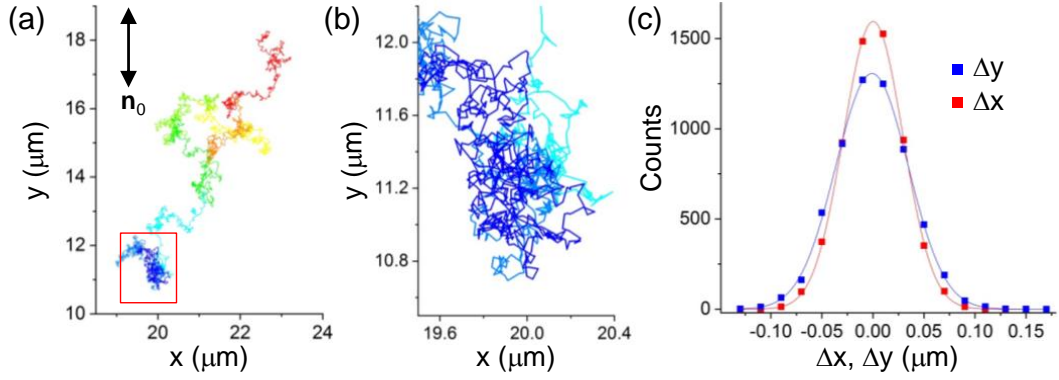

Figure S8. Diffusion of a single charged colloidal dumping in a nematic liquid crystal. **a** Large scale and **b** zoomed-in trajectory of Brownian motion of a charged colloidal dumping in a planar nematic cell. **c** Histograms of displacements along ( $y$  axis) and perpendicular ( $x$  axis) to  $\mathbf{n}_0$  for a colloidal dumping.

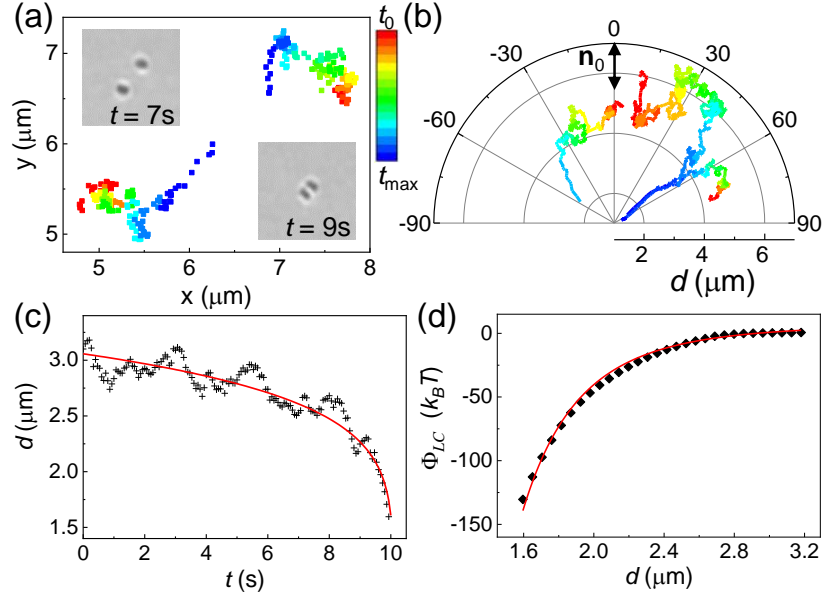

Figure S9. Elastic pair interactions of uncharged dumping particles. **a** Trajectories of two interacting particles; color shows the time with respect to color scale. **b** Polar plot of interacting particles released at different angles. **c** Time dependence of separation corresponding to (a). **d** Elastic interaction potential  $\Phi_{LC}$  extracted from (c), showing elastic quadrupole (red lines show  $1/d^5$  fit).

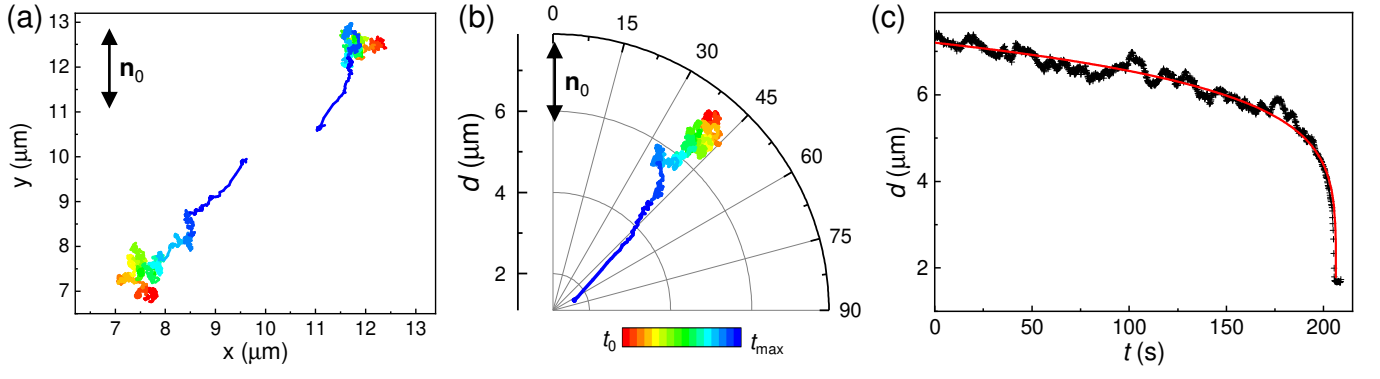

Figure S10. Pair interactions of weakly charged dumping particles in a nematic LC. **a** Trajectory of interactions between two weakly charged particles. **b** Polar plot of a separation depending on an angle  $\theta$  for two weakly charged particles; particles come to the direct contact at  $45^\circ$ - $60^\circ$ . **c** Time dependence of separation corresponding to **a** and **b**.
